# Supplementary material for: Rethinking Generic Object Tracking Toward Human-Level Perceptual Intelligence
Source: arXiv:2607.01395 source file (2026-07-01)
Supplement: Supplementary file 1 [file appendix.tex]

\paragraph{Sample PDF Complete} A simple inclusion of a PDF file. It will start on next page and be inserted. 
% Format command : \includepdf[page=-]{filename}
\includepdf[page=-]{Appendices/sample}

\paragraph{Sample PDF Only Page no.2} Only include the second page of a PDF file.It will start on next page and be inserted. 
% Format command : \includepdf[page={page number,page number,etc.}]{filename}
\includepdf[page={2}]{Appendices/sample}
